# Supplementary material for: Second-order perturbative correlation energy functional in the ensemble density-functional theory
Source: arXiv:2109.07697 source file (2021-10-26)
Supplement: Supplementary file 1 [file supplemental.pdf]

# Supplemental material for "Second-order perturbative correlation energy in the ensemble density-functional theory"

Zeng-hui Yang[1, 2]

[1] Microsystem and Terahertz research center, China Academy of Engineering Physics, Chengdu, China 610200
[2] Institute of Electronic Engineering, China Academy of Engineering Physics, Mianyang, China 621000

(Dated: October 26, 2021)

This supplemental material contains the derivation of the fixed-orbital $\mathtt{w}$-derivative $v_{\mathrm{Hx},\mathtt{w}}$ term in DEC/EEXX+PT2 calculations, DEC/EEXX+PT2 excitation energies of the 1D Hooke's atom and 1D charge-transfer box, and the convergence of DEC/PT2 excitation energies for the 1D flat box, the 1D charge-transfer box and the 3D He atom.

## I. DERIVATION OF THE OPTIMAL EFFECTIVE POTENTIAL OF EEXX

We derive the $v_{\mathrm{HX},\mathtt{w}}$ and its fixed-orbital $\mathtt{w}$-derivative in the following, which is needed by the second term of Eq. (31) of the main text. We only consider spin-unpolarized closed-shell system in the derivation for simplicity. The EEXX energy functional is

$$E_{\mathrm{Hx},\mathtt{w}} = \sum_{i=0}^{I}\sum_{k=1}^{g_i} w_{ik}\left\langle \Phi_{ik,w}\left|\hat{V}_{\mathrm{ee}}\right|\Phi_{ik,w}\right\rangle. \quad (1)$$

The notations are the same as in the main text. The potential of Eq. (1) can be derived by functional derivative as

$$v_{\mathrm{Hx},w}(\mathbf{r}) = \frac{\delta E_{\mathrm{Hx},w}[\{\phi_\mu\}]}{\delta n_w(\mathbf{r})} = \sum_{\mu}\int \mathrm{d}^3r'\mathrm{d}^3r''\frac{\delta E_{\mathrm{Hx},w}}{\delta\phi_\mu(\mathbf{r}')}\frac{\delta\phi_\mu(\mathbf{r}')}{\delta v_{\mathrm{s},w}(\mathbf{r}'')}\frac{\delta v_{\mathrm{s},w}(\mathbf{r}'')}{\delta n_w(\mathbf{r})} + \mathrm{c.c.}, \quad (2)$$

which can be rearranged into the OEP equation:

$$\int \mathrm{d}^3r'\, v_{\mathrm{Hx},w}(\mathbf{r}')\frac{\delta n_w(\mathbf{r}')}{\delta v_{\mathrm{s},w}(\mathbf{r})} = \int \mathrm{d}^3r'\sum_{\mu}\frac{\delta E_{\mathrm{Hx},w}}{\delta\phi_\mu(\mathbf{r}')}\frac{\delta\phi_\mu(\mathbf{r}')}{\delta v_{\mathrm{s},w}(\mathbf{r})} + \mathrm{c.c.} \quad (3)$$

We then evaluate the quantities in Eq. (3). $\delta\phi_\mu(\mathbf{r}')/\delta v_{\mathrm{s},w}(\mathbf{r})$ on the right hand side of Eq. (3) can be obtained from perturbation theory and have the same form as in ground-state OEP:

$$\frac{\delta\phi_\mu(\mathbf{r}')}{\delta v_{\mathrm{s},w}(\mathbf{r})} = \sum_{\nu\neq\mu}\frac{\phi_\nu^*(\mathbf{r})\phi_\mu(\mathbf{r})\phi_\nu(\mathbf{r}')}{\epsilon_\mu - \epsilon_\nu}. \quad (4)$$

$\delta n_w(\mathbf{r}')/\delta v_{\mathrm{s},w}(\mathbf{r})$ on the left hand side of Eq. (3) can be evaluated using the chain rule:

$$\frac{\delta n_w(\mathbf{r}')}{\delta v_{\mathrm{s},w}(\mathbf{r})} = \sum_{i=0}^{I}\sum_{k=1}^{g_i}\sum_{\mu\sigma}\int \mathrm{d}^3r'_1\ldots\mathrm{d}^3r'_N\mathrm{d}^3r'' \frac{\delta n_w(\mathbf{r}')}{\delta\Phi_{ik}(\mathbf{r}'_1,\ldots,\mathbf{r}'_N)}\frac{\delta\Phi_{ik}(\mathbf{r}'_1,\ldots,\mathbf{r}'_N)}{\delta\phi_{\mu\sigma}(\mathbf{r}'')}\frac{\phi_{\mu\sigma}(\mathbf{r}'')}{\delta v_{\mathrm{s},w}(\mathbf{r})} + \mathrm{c.c.}, \quad (5)$$

where $\sigma$ denotes the spin. Although we only consider closed-shell systems, the spin need to occur explicitly here since they cannot be ignored in the Slater determinant. The first term in Eq. (5) is

$$\frac{\delta n_w(\mathbf{r}')}{\delta\Phi_{ik}(\mathbf{r}'_1,\ldots,\mathbf{r}'_N)} = w_{ik}\Phi_{ik}^*(\mathbf{r}'_1,\ldots,\mathbf{r}'_N)\sum_{a=1}^{N}\delta(\mathbf{r}'-\mathbf{r}_a). \quad (6)$$

The second term in Eq. (5) can be written as

$$\frac{\delta\Phi_{ik}(\mathbf{r}'_1,\ldots,\mathbf{r}'_N)}{\delta\phi_{\mu\sigma}(\mathbf{r}'')} = \sum_p C_{ikp}\frac{\delta\tilde{\Phi}_{\tilde{i}p}(\mathbf{r}'_1,\ldots,\mathbf{r}'_N)}{\delta\phi_{\mu\sigma}(\mathbf{r}'')} = \sum_p C_{ikp}\left[\tilde{\Phi}_{\tilde{i}p}\right]_{\mu\sigma}^{\delta\sigma}(\mathbf{r}'_1,\ldots,\mathbf{r}'_N,\mathbf{r}''), \quad (7)$$

where the notation $\left[\tilde{\Phi}_{\tilde{i}p}\right]_{\mu\sigma}^{\delta\sigma}(\mathbf{r}'_1,\ldots,\mathbf{r}'_N,\mathbf{r}'')$ means that the column with $\phi_{\mu\sigma}$ in the Slater determinant are replaced by Dirac $\delta$ functions $\delta(\mathbf{r}''-\mathbf{r}_1)$, $\delta(\mathbf{r}''-\mathbf{r}_2)$ and so on multiplied by the spin function corresponding to $\sigma$. The third term in Eq. (5) is Eq. (4), and $\sigma$ can be omitted. The full formula for $\delta n_w(\mathbf{r}')/\delta v_{\mathrm{s},w}(\mathbf{r})$ is then

$$\frac{\delta n_w(\mathbf{r}')}{\delta v_{\mathrm{s},w}(\mathbf{r})} = \sum_{i=0}^{I}\sum_{k=1}^{g_i} w_{ik}\sum_{p,q=1}^{g_{\tilde{i}}} C_{ikp}C_{ikq}^*\sum_{\mu\sigma,\nu\neq\mu} \frac{\phi_\nu^*(\mathbf{r})\phi_\mu(\mathbf{r})}{\epsilon_\mu-\epsilon_\nu}\left\langle\tilde{\Phi}_{\tilde{i}q}\left|\hat{n}(\mathbf{r}')\right|\left[\tilde{\Phi}_{\tilde{i}p}\right]_{\mu\sigma}^{\nu\sigma}\right\rangle + \mathrm{c.c.}, \quad (8)$$

where $\left[\tilde{\Phi}_{\tilde{i}p}\right]_{\mu\sigma}^{\nu\sigma}$ denotes the Slater determinant obtained by replacing $\phi_{\mu\sigma}$ in $\tilde{\Phi}_{\tilde{i}p}$ with $\phi_{\nu\sigma}$.

The $\hat{n}(\mathbf{r}')$ matrix elements in Eq. (8) prevents the OEP equation from further simplification. In the following, we approximate Eq. (8) by only considering the $p = q$ terms, so that the OEP equation can be reduced to a form similar to its ground-state counterpart. Eq. (3) then becomes

$$\sum_{i=0}^{I}\sum_{k=1}^{g_i} w_{ik}\sum_{p=1}^{\tilde{g}_{\tilde{i}}} C_{ikp}\sum_{\mu\sigma} f_{\tilde{i}p\mu\sigma}\int \mathrm{d}^3r'\left[C^*_{ikp}v_{\mathrm{Hx},w}(\mathbf{r}') - \sum_{q=1}^{\tilde{g}_{\tilde{i}}} C^*_{ikq}\mathcal{V}_{\tilde{i}pq\mu\sigma}(\mathbf{r}')\right]\sum_{\nu\neq\mu}\frac{\phi^*_\nu(\mathbf{r})\phi_\mu(\mathbf{r})\phi^*_\mu(\mathbf{r}')\phi_\nu(\mathbf{r}')}{\epsilon_\mu-\epsilon_\nu} + \text{c.c.} = 0, \quad (9)$$

where

$$\mathcal{V}_{\tilde{i}pq\mu\sigma}(\mathbf{r}') = \frac{1}{\phi^*_{\mu\sigma}(\mathbf{r}')}\frac{\delta\left\langle \tilde{\Phi}_{\tilde{i}q}\middle|\hat{V}_{\mathrm{ee}}\middle|\tilde{\Phi}_{\tilde{i}p}\right\rangle}{\delta\phi_{\mu\sigma}(\mathbf{r}')}, \quad (10)$$

and $f_{\tilde{i}p\mu\sigma}$ is the occupation number of $\phi_{\mu\sigma}$ in Slater determinant $\tilde{\Phi}_{\tilde{i}p}$. Detailed formulas for evaluating Eq. (10) can be derived using Slater-Condon rules.

A Krieger-Li-Iafrate (KLI)[1] type approximation to $v_{\mathrm{Hx,w}}$ can be obtained from Eq. (9):

$$v^{\mathrm{KLI}}_{\mathrm{Hx},w}(\mathbf{r}) = \frac{1}{2\rho_w(\mathbf{r})}\sum_{i=0}^{I}\sum_{k=1}^{g_i} w_{ik}\sum_{p=1}^{\tilde{g}_{\tilde{i}}} C_{ikp}\sum_{\mu\sigma} f_{\tilde{i}p\mu\sigma}n_\mu(\mathbf{r})\left\{\sum_{q=1}^{\tilde{g}_{\tilde{i}}} C^*_{ikq}\mathcal{V}_{\tilde{i}pq\mu\sigma}(\mathbf{r}) + \left[C^*_{ikp}\bar{v}_{\mathrm{Hx},w,\mu} - \sum_{q=1}^{\tilde{g}_{\tilde{i}}} C^*_{ikq}\bar{\mathcal{V}}_{\tilde{i}pq\mu\sigma}\right]\right\} + \text{c.c.}, \quad (11)$$

where

$$\rho_w(\mathbf{r}) = \sum_{i=0}^{I}\sum_{k=1}^{g_i} w_{ik}\sum_{p=1}^{\tilde{g}_{\tilde{i}}} |C_{ikp}|^2\sum_{\mu\sigma} f_{\tilde{i}p\mu\sigma}n_\mu(\mathbf{r}), \quad (12)$$

$$\bar{v}_{\mathrm{Hx},w,\mu} = \int \mathrm{d}^3r' v_{\mathrm{Hx},w}(\mathbf{r}')n_\mu(\mathbf{r}'), \quad (13)$$

$$\bar{\mathcal{V}}_{\tilde{i}pq\mu\sigma} = \int \mathrm{d}^3r'\mathcal{V}_{\tilde{i}pq\mu\sigma}(\mathbf{r}')n_\mu(\mathbf{r}'), \quad (14)$$

with $n_\mu(\mathbf{r}) = |\phi_\mu(\mathbf{r})|^2$. Although Eq. (13) and (14) can be solved using linear algebra, its $\mathtt{w}$-dependence becomes very complicated, and we are unable to obtain a general closed-form expression for $\partial v_{\mathrm{Hx,w}}[n_{\mathrm{s,w}}[\{\phi_\mu\}]]/\partial \mathtt{w}$ required by the DEC method. We therefore use a Slater-type approximation[2] in the following calculation for Be with both $\bar{v}_{\mathrm{Hx},w,\mu}$ and $\bar{\mathcal{V}}_{\tilde{i}pq\mu\sigma}$ set to zero:

$$v^{\mathrm{Slater}}_{\mathrm{Hx},w}(\mathbf{r}) = \frac{1}{2\rho_w(\mathbf{r})}\sum_{i=0}^{I}\sum_{k=1}^{g_i} w_{ik}\xi_{ik}(\mathbf{r}) + \text{c.c.}, \quad (15)$$

where

$$\xi_{ik}(\mathbf{r}) = \sum_{p,q=1}^{\tilde{g}_{\tilde{i}}} C_{ikp}C^*_{ikq}\sum_{\mu\sigma} f_{ip\mu\sigma}\phi_\mu(\mathbf{r})\frac{\delta\left\langle \tilde{\Phi}_{\tilde{i}q}\middle|\hat{V}_{\mathrm{ee}}\middle|\tilde{\Phi}_{\tilde{i}p}\right\rangle}{\delta\phi_{\mu\sigma}(\mathbf{r})}. \quad (16)$$

The fixed-orbital $\mathtt{w}$-derivative of Eq. (15) is

$$\left.\frac{\partial v^{\mathrm{Slater}}_{\mathrm{Hx},w}[n_{\mathrm{s},w}[\{\phi_\mu\}]](\mathbf{r})}{\partial w}\right|_{\phi_\mu=\phi^{\mathrm{KS}}_{\mu,w}} = \frac{1}{2\rho_w(\mathbf{r})}\sum_{i=0}^{I}\sum_{k=1}^{g_i}\frac{\partial w_{ik}}{\partial w}\xi_{ik}(\mathbf{r}) - \frac{1}{2\rho_w(\mathbf{r})}\frac{\partial\rho_w(\mathbf{r})}{\partial w}\sum_{i=0}^{I}\sum_{k=1}^{g_i} w_{ik}\xi_{ik}(\mathbf{r}) + \text{c.c.} \quad (17)$$

## II. DEC/EEXX+PT2 EXCITATION ENERGIES FOR 1D HOOKE'S ATOM AND 1D CHARGE-TRANSFER BOX

The DEC/EEXX+PT2 excitation energies for 1D Hooke's atom and 1D charge-transfer box are listed in Table I.

| $I$ | $\omega_I^{\mathrm{exact}}$ | $\omega_I^{\mathrm{PT2}}$ (H) |
|---|---|---|
| 1D Hooke's atom | | |
| 1 | 1.0000 | 1.0022 |
| 2 | 1.9640 | 1.9685 |
| 3 | 2.0000 | 1.9964 |
| 4 | 2.9640 | 2.9822 |
| 5 | 3.0000 | 2.9824 |
| 1D charge-transfer box | | |
| 1 | 1.1307 | 1.1308 |

TABLE I. DEC/EEXX+PT2 excitation energies for 1D Hooke's atom (singlet only) and 1D charge-transfer box. The calculations are the same as those in the main text.

## III. CONVERGENCE OF DEC/EEXX+PT2 IN 1D FLAT BOX, 1D CHARGE-TRANSFER BOX AND 3D HE ATOM

Convergence curves for PT2 in 1D flat box, 1D charge-transfer box and 3D He atom are plotted in Figs. 1, 2 and 3.

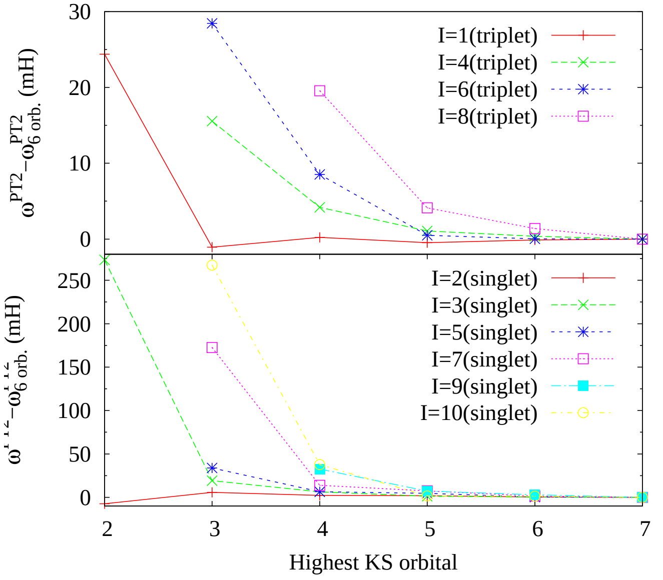


FIG. 1. Convergence of DEC/EEXX+PT2 excitation energies of the 1d flat box with respect to the number of KS orbitals included in the calculation.

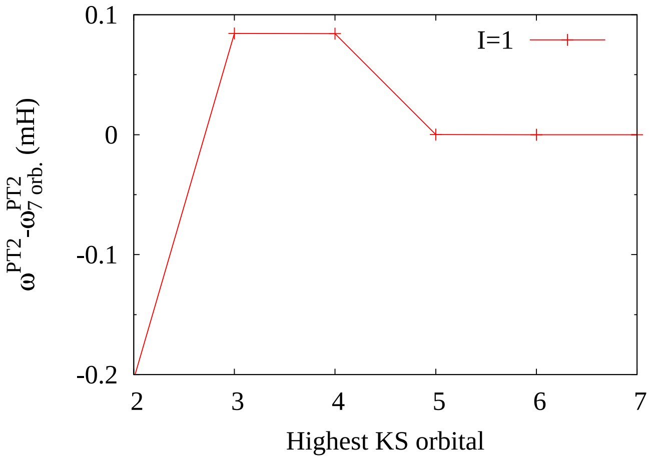


FIG. 2. Convergence of DEC/EEXX+PT2 first excitation energy of the 1d charge-transfer box with respect to the number of KS orbitals included in the calculation.

[1] J. B. Krieger, Y. Li, and G. J. Iafrate. Construction and application of an accurate local spin-polarized kohn-sham potential with integer discontinuity: exchange-only theory. *Phys. Rev. A*, 45:101, 1992.
[2] C. A. Ullrich. *Time-Dependent Density-Functional Theory: Concepts and Applications.* Oxford University Press, Oxford, 2012.

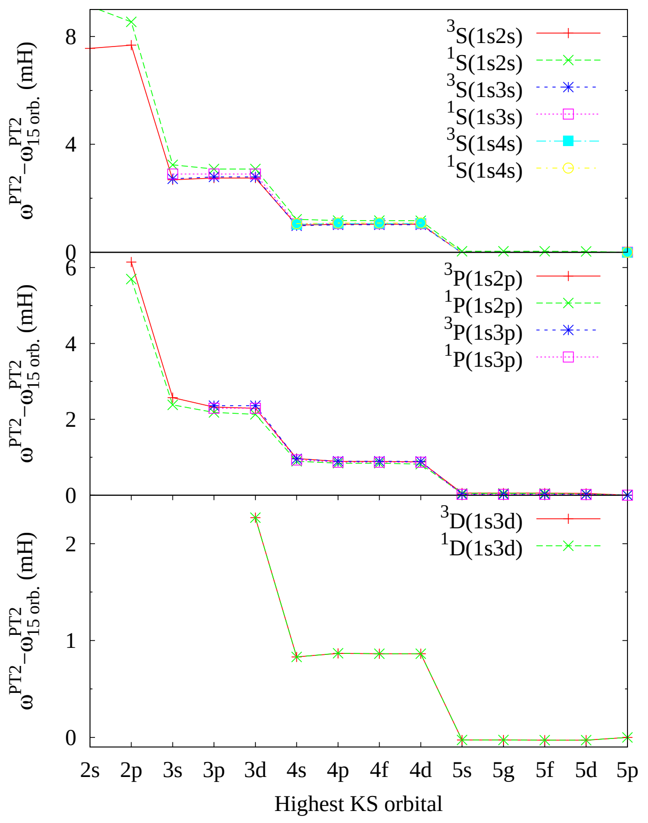


FIG. 3. Convergence of DEC/EEXX+PT2 excitation energies of the He atom with respect to the number of KS orbitals included in the calculation.
